# Supplementary material for: Proof-of-Authorship for Diffusion-based AI Generated Content
Source: arXiv:2603.17513 source file (2026-09-21)
Supplement: Supplementary file 1 [file changes_appendix.tex]

\section{Summary of Changes Made for Minor Revision}
\label{app:changes}


We thank the reviewers for their constructive feedback, and have used these feedback to improve the manuscript's quality. 
{\color{blue}
The main additions are highlighted in blue, with their corresponding description below.  
 
\subsection*{Item (1): Strengthening the theoretical justification for Assumption A2 and clarifying the role of optimization-based attacks under the cryptographic reduction}
 
\begin{itemize}
    \item \textbf{Justification for A2.} The assumption is explicitly stated in Section \ref{sec:assumption}, and the justification is in Section \ref{section:A2-analysis}. In particular, we give
    \begin{enumerate}
        \item A sufficient condition for A2 to occur (A2-I) that individual coordinates in the generated latent follow a sub-Gaussian distribution. 
        \item Show in Lemma \ref{lemma:subexp} that A2-I is a sufficient condition for A2. 
        \item Listed evidence supporting A2-I in Section \ref{section:A2-analysis} 
        \item Although not required to prove A2, we show that under a slightly stronger weak dependence condition (A2-II), we can obtain a sharper $\exp(-\widetilde{\Omega}(d)\,t)$ tail probability bound.  Nonetheless, Remark \ref{remark:subexp_bernstein} and Appendix~\ref{app:stronger-tail}  states explicitly that this bound is supplementary: Lemma~\ref{lemma:subexp} is already sufficient to show A2 holds.
    \end{enumerate}

    \item \textbf{Empirical assessment of (A2-I) and (A2-II).} The new Section~\ref{section:sub-exp-tail}  assesses both (A2-I) and (A2-II) on SD~2.1 and SD~XL, with empirical evidence supporting (A2-I) and (A2-II) in both models. 
    \item \textbf{Role of optimization-based attacks.} Section~\ref{subsubsection:adaptive_forger} explains why the PRF defeats adaptive/optimization-based attacks, and relates it to the reduction in Theorem \ref{thm:poa_PPT}'s proof. 
    % Complementing the reduction, the new Appendix~I.2 empirically evaluates a regeneration attack~\cite{zhao2024regeneration}, with an attack success rate of 0\% on both SD~2.1 and SD~XL at $p_r = 2^{-50}$, and Section~4.5 analyzes worst-case $\ell_p$-bounded adversarial perturbations of the similarity function (Appendix~H).
\end{itemize}
 
\subsection*{Item (2): Revising the security claims, in particular the reported forgery probability}
 
\begin{itemize}
    \item \textbf{Separation of cryptographic and statistical guarantees.} The revision distinguishes throughout between (i) the cryptographic guarantee (Theorem~\ref{thm:poa_PPT}: no PPT forger outperforms a random forger, relying on A1 only) and (ii) estimating random forger's success probability $q$, which additionally relies on A2 for extremely small $q$.
    \item \textbf{Direct validation of the tail extrapolation.} The new
    Section~\ref{subsection:tail_validation} validates the extrapolation: a distribution fitted under Assumption A2 on $2^{10}$ samples
    (the PA's sample size) is compared against empirical tail frequencies
    from $2^{17}$ independent samples. In our evaluations, the upper confidence bound (the quantity actually used by the
    judge) overestimates the tail probability in every case, erring on
    the side of rejecting forgeries. The section states the limitation
    explicitly: validation extends to the $2^{-17}$ quantile, and deeper
    validation remains conditional on the parametric form.
    \item \textbf{Calibrated claim language.} The claims have been reworded across the paper to reflect their assumption dependence: 
    \begin{enumerate}
        \item Section \ref{sec:assumption}: Explains the role of A1 and A2, i.e. A2 is used to estimate tail probability $q$ with polylog samples, instead of $1/q$ samples.
        \item Section \ref{sec:distribution-free}: States how adjudication is performed without assuming A2, i.e. while $q= 2^{-50}$ is unattainable certification is still possible for moderate values of $q$ like $2^{-10}$ or $2^{-20}$
        \item Section \ref{sec:securityanalysis}: We reorganized security analysis section, including how the framework rules out optimization-based forgers and backdoored models, to make it explicit that it relies solely on A1 (and not A2). 
      \item Section~\ref{subsection:tail_validation} states explicitly
      that empirical validation extends only to the $2^{-17}$ quantile,
      with deeper extrapolation conditional on the parametric form.
      \item Caption in Figure 1 states that the $2^{-50}$   bound holds under the assumptions of
Section~\ref{sec:assumption}.
    \end{enumerate}
    
    
    % \item \textbf{Distribution-free fallback.} The new Section~\ref{sec:distribution-free} gives a verification procedure that avoids parametric tail extrapolation entirely, certifying $q \le \ln(1/\delta)/n$ from $n$ samples with no distributional assumption. This certifies moderate levels (e.g., $2^{-10}$, $2^{-20}$) assumption-free and delimits what is and is not attainable without A2; the judge's options when A2 cannot be supported are stated at the end of Section~4.4.2.
\end{itemize}
 
\subsection*{Item (3): Clarifying the requirement of access to the original model for verification}
 
\begin{itemize}
    \item Section~\ref{subsection:practical} (``Model Availability During Adjudication'') now states the requirement and its implications explicitly: authors should archive the exact model and generation pipeline; for proprietary models, verification may be performed by a trusted PA with confidential model access while all other information remains public; and if the original model is unavailable, a claim is {unverifiable} under our framework rather than invalid. 
\end{itemize}


 }
\subsection*{Additional changes in response to reviewer comments}

\begin{itemize}
    \item \textbf{Additional evaluations.} All evaluations now include SD~XL alongside SD~2.1, with similar results as previously reported on SD 2.1. {\color{blue} Added a regeneration attack evaluation in Section \ref{section:eval_regen}, with similar results to those reported previously in Sections \ref{section:eval_robust} (JPEG compression, Gaussian noise, etc.)}
     {\color{blue} 
    \item \textbf{Independent generations leading to ambiguity.}
    Remark~\ref{remark:independent_honest_generation} addresses whether
    two users who independently generate similar images could both
    obtain sufficiently small $q$-values: by Assumption~A1 and
    Lemma~\ref{lemma:subexp}, such collisions occur with only
    exponentially small probability.
    \item \textbf{Role of the public ledger.}
Section~\ref{subsection:practical} clarifies that a public ledger and POA are
complementary: ledger timestamping alone gives proof-of-ownership,
while POA adds proof-of-authorship, with the ledger serving optionally
as a channel for broadcasting identities. 

    }
    \item \textbf{Comparison with seed-based provenance.} Sections~\ref{subsubsection:seed_based} and~\ref{subsection:seed_based_vs_poa} add an explicit comparison with NoisePrints~\cite{goren2025noiseprintsdistortionfreewatermarksauthorship} along three axes: secret-free public verification, reproduction-based rather than correlation-based grounding, and quantified probabilistic adjudication versus threshold-based binary acceptance.
    \item \textbf{Presentation.} We thank reviewer A's feedback regarding subcaptions (a)--(c) in Figure 1 and Table captions, they have been fixed in this version.  Further presentation changes are
    \begin{enumerate}
        \item Improved the technical explainations, e.g. the part on cryptographic reduction argument for the forger.
        \item Moved some evaluations from the main body to appendix (i.e. evaluations in Appendix \ref{subsection:seed_induced} and \ref{section:expt_sim}). This is done due to space constraints, in favour of the new experiments introduced. 
    \end{enumerate}
     We emphasize that these changes do not alter the findings and main results, they are to improve the manuscript's readability and presentation. 
\end{itemize}
 
